# Supplementary material for: How Well Sensing Integrates with Communications in MmWave Wi-Fi?
Source: arXiv:2302.08378 source file (2023-02-16)
Supplement: Supplementary file 1 [file code.tex]

\chapter{Software}\label{app:software}

\begin{lstlisting}[language=Arduino]  


\end{lstlisting}
