# Supplementary material for: How Well Sensing Integrates with Communications in MmWave Wi-Fi?
Source: arXiv:2302.08378 source file (2023-02-16)
Supplement: Supplementary file 2 [file equations.tex]

\chapter{An example of an appendix}
